# Supplementary material for: Linearized theory of the fluctuation dynamics in 2D topological lasers
Source: arXiv:2101.11737 source file (2021-09-20)
Supplement: Supplementary file 1 [file appendix.tex]

\subsubsection{Reverse chirality modes:}

Another strength of this 1D effective model is that it can also predict the shape of the branch of excitations resulting from the chiral edge modes of opposed chirality, namely in the gap opposed to the one containing the lasing mode (situated around $k= -\pi$ and $k=\pi$ in the elementary excitations spectrums). We call these excitations Reverse Chirality Modes, whose importance will be clear in the following. 

To do so, it is necessary to remark that the edge modes of the bottom gap lie in a separated wavevector interval ($k_y \in [-\pi, 0]$) than the ones of the upper gap ($k_y \in [0,\pi]$). Then, setting the function:

\begin{equation}\label{eq:2.10}
\epsilon(k_y) =
    \left\{
    \begin{array}{ll}
        \epsilon_{bot}(k_y) & \mbox{if } k_y \in [-\pi, 0] \\
        \epsilon_{top}(k_y) & \mbox{if } k_y \in [0, \pi]
    \end{array}
\right.
\end{equation}

and same for $G(k_y)$ is a sufficient operation to retrieve the shape of the reverse chirality modes branches of excitations, as plotted in Fig. \ref{fig3}.

Finally, the advantage of deriving this 1D effective model is that it allows to compute in a very simple way the elementary excitations spectrums, as it does not require to make a time-evolution simulation of the system every time a parameter is changed. 

\begin{figure}[h]
    \centering
    \includegraphics[scale=0.21]{comparaison_lowqual.png}
    \caption{Comparisons of the real (left) and imaginary (right) part of the elementary excitations spectrums between the full 2D model and the 1D approximate models. Dark color scale indicates the excitations calculated with the full 2D model. Red (green) color scale indicates the excitations calculated with the effective 1D model (1D gGPE). 
    Panels (a)-(e), same parameters as in Fig. \ref{fig2} (a) but: $\gamma_R = \gamma$ in (b), $k_{y,0} = -1.456$ in (c), $\frac{g_R}{R} = -3$ in (d) and $\gamma = 1J$ in (e). The $G^{nh}$ function is used in (d),(e).}
    \label{fig3}
\end{figure}

APPENDIX...

However, this last formula is not dependent on the linewidth enhancement factor which makes clear that it is not able to capture the asymmetry of the gain curve. It means that the modifications of the spectrum due to the non hermitian part of (\ref{eq:2.2}) are becoming significant, making the $G(k_y)$ function inaccurate. Similarly, in the case of high pump intensities, there is no asymmetry but the lasing threshold becomes lower. 

Nevertheless, an approximation of $G$ can be found, replacing $G$ by:

\begin{equation}\label{eq:2.100}
    G^{nh}(k_y) =
    \left\{
    \begin{array}{ll}
        \frac{\gamma}{G_{max} P^{th, bot}} G(k_y) & \mbox{if } k_y \in [-\pi, 0] 
        \\ 
        \\
        \frac{\gamma}{G_{max} P^{th, top}} G(k_y) & \mbox{if } k_y \in [0, \pi]
    \end{array}
\right.
\end{equation}

where $G_{max}= max(G) = 0.876$, $P^{th, bot}$ ($P^{th, top}$) is the pumping intensity at threshold for the bottom (top) gap, calculated as in Sec 2 A. An estimation of the $P^{th, bot/top}(\gamma, g_R)$ functions is given in Appendix A.

It amounts to assess that the good overlap function has same shape as the one from the bare Harper-Hofstadter eigenstates but different amplitude in each gap, which can be evaluated by the threshold value. Finally, comparison with results from (\ref{eq:2.4}) is shown in Fig. \ref{fig1} (d), exhibiting a good agreement.
